# Supplementary material for: "How to best say it?" : Translating Directives in Machine Language into Natural Language in the Blocks World
Source: arXiv:2107.06886 source file (2021-07-14)
Supplement: Supplementary file 1 [file 8_appendix.tex]

\section{Appendix}

\begin{table*}[t]
\resizebox{\textwidth}{!}{%
\begin{tabular}{@{}llllll@{}}
\toprule
step  & directive                                                            & depth & \#prop & cost1 & cost2 \\ \midrule
a & Put a block on the table.                                            & 1     & 2      & 0.135 & 0.158 \\
b & Put a block on top of it.                                            & 1     & 2      & 0.135 & 0.096 \\
  & Put a block on top of the block you just placed.                     & 1     & 3      & 0.144 & 0.117 \\
c & Put a block behind the stack.                                        & 1     & 2      & 0.135 & 0.158 \\
  & Put a block behind the stack you just made.                          & 1     & 3      & 0.144 & 0.117 \\
  & Put a block behind the block at the bottom.                          & 2     & 3      & 0.183 & 0.246 \\
d & Put a block to the right of it.                                      & 1     & 2      & 0.135 & 0.096 \\
  & Put a block to the right of the previous block.                      & 1     & 3      & 0.144 & 0.117 \\
  & Put a block to the right of the block at the back.                   & 2     & 3      & 0.183 & 0.246 \\
e & Put a block behind the stack.                                        & 1     & 2      & 0.135 & 0.158 \\
  & Put a block behind the block on the top.                             & 2     & 3      & 0.183 & 0.245 \\
  & Put a block on top of the block that is at the back and on the left. & 3     & 4      & 0.210 & 0.342 \\
f & Add one more.                                                        & 0     & 1      & 0.117 & 0.039 \\
  & Put a block on top of it.                                            & 1     & 2      & 0.135 & 0.096 \\
  & Put a block on top of the same stack.                                & 1     & 3      & 0.144 & 0.117 \\
  & Put a block on top of the stack at the back.                         & 2     & 3      & 0.183 & 0.246 \\
  & Put a block on top of the block that is on the top and at the back.  & 3     & 4      & 0.210 & 0.342 \\ \bottomrule
\end{tabular}%
}\caption{\label{tab:plan_speech_result_full} Plan description speeches generated for all steps in Figure \ref{fig:plan_example1}.}
\end{table*}

\subsection{Additional Result}
Table~\ref{tab:plan_speech_result_full} expanded result presented in Table~\ref{tab:plan_speech_result}. Directives generated for each step in Figure~\ref{fig:plan_example1}.

\subsection{Visualization of predicate evaluation}
Visualization of predicate fields described in section~\ref{sec:spatialRelationship}.

\begin{figure}[h]
\includegraphics[width=0.5\textwidth]{figures/predicatefields_1row.png}
\caption{\textbf{Visualization of predicate fields for Spatial Relationship Evaluation} Shaded blue boxes represent valid space with probability (darker is lower) for predicates: (a) in front of the bottom block of the stack, (b) in front of the stack, (c) on top of the stack, (d) corner of the table.}
\label{fig:predicateFields}
\end{figure}
